# Supplementary material for: Resilient Edge: Can we achieve Network Resiliency at the IoT Edge using LPWAN and WiFi?
Source: arXiv:2205.03729 source file (2022-05-07)
Supplement: Supplementary file 1 [file appendix.tex]

\subsection{Functions provided by PyCom}
\textbf{LoRa}
Pycom Micropython LoRa\footnote{LoRa Firmware API \url{https://docs.pycom.io/firmwareapi/pycom/network/lora/}} provides functions to provide information about the bandwidth, coding rate, spreading factor, connection status, time-on-air (milisec) for the current Lora settings, and stats (such as RSSI) from the last received packet respectively. The coding rate refers to the proportion of transmitted bits that carry information. With regards to range, TX power can be increased. Further, the SF/data rate can also be changed. The slower the data rate (higher number SF, like SF12), the longer the range is supposed to be. slower coding allows to detect the signal in the background noise. Information is transferred for a longer time with a well structured signal which is different to a random noise. Interesting thread on real range of LoRaWAN\footnote{\url{https://forum.pycom.io/topic/6102/what-is-the-realistic-range-of-lorawan/2}}. Notes on setting spreading factor\footnote{\url{https://forum.pycom.io/topic/6103/set-spreading-factor}} Lora Source code\footnote{Pycom-sigfox directory: .../esp32/mods/modlora.c as entry point for the python API Supporting code: .../lib/lora/......./drivers/sx27x/... .../esp32/lora/....}

\textbf{SigFox}
Pycom Micropython SigFox\footnote{Sigfox Firmware API \url{https://docs.pycom.io/firmwareapi/pycom/network/sigfox/}} provides functions to determine frequencies (download frequency and upload frequency) and RSSI based on the last downlink message received.

\textbf{LTE}
Pycom Micropython LTE\footnote{LTE Firmware API \url{https://docs.pycom.io/firmwareapi/pycom/network/lte/}} provides functions for attaching, detaching to the LTE network, check whether attached; connect, disconnect, isconnected to start a data session and check whether connected to the network; pppsuspend and pppresume to suspend PPP session with LTE modem and send AT commands. Further functions ue\_coverage, psm provides information about NB-IoT coverage and power saving mode settings. Further, AT command\footnote{Monarch Platform AT Commands \url{https://nimbelink.com/Documentation/Skywire/4G_LTE_Cat_M1/1001534_NL-SW-LTE-SVZM_AT_COMMAND_MANUAL.pdf}} 'AT+CSQ' provides the received signal strength indication (rssi) and
channel bit error rate (ber).

\textbf{Wi-Fi}
Pycom Micropython WLAN\footnote{WLAN Firmware API \url{https://docs.pycom.io/firmwareapi/pycom/network/wlan/}} provides functions to scan, connect, disconnect to the network. Further, it also provides a function to set the bandwidth of the wifi, either 20 MHz or 40 MHz. Also, it allows to set FiPy in three WLAN modes: station, access point and Station with Access point. FiPy can be set as a Access Point and in station mode. \notevk{Check if it can be set into both mode and can route data from stations connected to AP. This can be used to extend the Wi-Fi} and can connect over WEP, WPA, WPA2 and WPA2-Enterprise.
